# Supplementary material for: Foundations of Symbolic Languages for Model Interpretability
Source: arXiv:2110.02376 source file (2021-11-14)
Supplement: Supplementary file 1 [file appendix.tex]

\subsection{Review of First Order Logic} 

We quickly review the definition of First Order Logic (\FO) over vocabularies without function symbols.

\paragraph{Syntax of \FO.} A {\em vocabulary} $\sigma$ is a finite list 
$(R_1,\dots,R_m,c_1,\dots,c_p)$, where each $R_i$ is a relation symbol with associated arity $n_i > 0$, for $i \in [1,m]$, and each $c_j$ is a constant symbol, 
for $j \in [1,p]$. We assume the existence of a countably infinite set of variables $\{x,y,z,\dots\}$, possibly with subscripts. 
A {\em $\sigma$-term} is either a variable or a constant symbol $c_j$, for $j \leq p$. The set $\FO[\sigma]$ 
of {\em \FO-formulas over $\sigma$} is inductively defined as follows. 
\begin{enumerate}
\item If $t_1,t_2$ are $\sigma$-terms, then $t_1 = t_2 \in \FO[\sigma]$.
\item If relation symbol $R_i$ has arity $n > 0$ and $t_1,\dots,t_n$ are $\sigma$-terms, then $R(t_1,\dots,t_n) \in \FO[\sigma]$.
\item If $\phi,\psi \in \FO[\sigma]$, then $\neg \phi$, $\phi \vee \psi$, and $\phi \wedge \psi$ also belong to $\FO[\sigma]$. 
\item If $x$ is a variable and $\phi \in \FO[\sigma]$, then $\exists x \phi$ and $\forall x \phi$ are in $\FO[\sigma]$.  
\end{enumerate}
\FO-formulas of type (1) and (2) are called {\em atomic}. A variable $x$ in $\FO$-formula $\phi$ appears {\em free}, if there is an occurrence of $x$ in $\phi$ that is not in the scope of a quantifier 
$\exists x$ or $\forall x$. 
A {\em $\FO$-sentence}  is a $\FO$-formula without free variables. We often write $\phi(\bar x)$ to denote that $\bar x$ is a tuple containing all free variables 
appearing in $\phi$. 

\paragraph{Semantics of \FO.} Formulas in $\FO[\sigma]$ are interpreted over {\em $\sigma$-structures}. Formally, a $\sigma$-structure is an ordered 
tuple 
$$\astruct \ = \ \langle A,\,R_1^\astruct,\cdots,R_m^\astruct,\,c_1^\astruct,\cdots,c_p^\astruct \rangle,$$ 
where $A$ is the {\em domain} of $\astruct$, for each relation symbol $R_i$ of arity $n$ ($i \leq m$) we have that $R_i^\astruct$ is an $n$-ary relation over $A$, and each $c_j^\astruct$ (for $j \leq p$) corresponds to 
an element in $A$. We call $R_i^\astruct$ and $c_j^\astruct$ the {\em interpretation} of $R_i$ and $c_j$ in $\astruct$, respectively. 
%We sometimes write $\dom(\astruct)$ for the domain of $\astruct$. 

Let $\phi(\bar x)$ be a formula in $\FO[\sigma]$ and $\astruct$ a $\sigma$-structure as defined above. 
Consider a mapping $\nu$ that associates an element in $A$ with each variable in $\bar x$ appearing free in $\phi$. 
We extend $\nu$ to the set of constant symbols in $\{c_1,\dots,c_p\}$ by setting $\nu(c_i) = c_i^A$. 
We formally define the {\em satisfaction of $\FO$-formula $\phi$ over the pair $(\astruct,\nu)$}, which we denote $(\astruct,\nu) \models \phi$, as follows.  
\begin{enumerate}
\item If $\phi$ is of the form $t_1 = t_2$, for $t_1,t_2$ $\sigma$-terms, then 
$(\astruct,\nu) \models \phi \, \Leftrightarrow \, \nu(t_1) = \nu(t_2)$. 
\item If $\phi$ is of the form $R_i(t_1,\dots,t_n)$, for $t_1,\dots,t_n$ $\sigma$-terms, then 
$(\astruct,\nu) \models \phi \, \Leftrightarrow \, \big(\nu(t_1),\dots,\nu(t_n)\big) \in R_i^\astruct$. 
\item If $\phi$ is of the form $\neg \psi$, then 
$(\astruct,\nu) \models \phi \, \Leftrightarrow \, (\astruct,\nu) \not\models \psi$.
 \item If $\phi$ is of the form $\psi \vee \psi'$, then 
$(\astruct,\nu) \models \phi$ iff $(\astruct,\nu) \models \psi$ or $(\astruct,\nu) \models \psi'$.
 \item If $\phi$ is of the form $\psi \wedge \psi'$, then 
$(\astruct,\nu) \models \phi$ iff $(\astruct,\nu) \models \psi$ and $(\astruct,\nu) \models \psi'$.
\item If $\phi$ is of the form $\exists x \psi$, then $(\astruct,\nu) \models \phi$ iff there exists $a \in A$ for which 
$(\astruct,\nu[x/a]) \models \psi$. Here, $\nu[x/a]$ is an assignment that takes the same value as $\nu$ 
on every variable $y \neq x$, and takes value $a$ on $x$. 
\item If $\phi$ is of the form $\forall x \psi$, then $(\astruct,\nu) \models \phi$ iff for every $a \in A$ we have that 
$(\astruct,\nu[x/a]) \models \psi$.
\end{enumerate}

For a \FO-formula $\phi(x_1,\dots,x_n)$ and assignment $\nu$ such that $\nu(x_i) = a_i$, for each $i \leq n$,  
we  write $\astruct \models \phi(\bar a)$, for $\bar a = (a_1,\dots,a_n)$, 
to denote that $(\astruct,\nu) \models \phi$. 
If $\phi$ is a sentence, we write simply $\astruct \models \phi$ to denote $(\astruct,\nu : \emptyset \to A) \models \phi$.

\newcommand{\D}{{\cal D}}

Before starting we define several important \FO-formulas over the vocabulary containing only the relation symbol $\subseteq$.
We use $\bar u,\bar v,\bar w,\dots$ to denote variables used by such formulas and which are interpreted over tuples in $\{0,1,\bot\}^t$, for some $t > 0$. 
If $\bar a \in \{0,1,\bot\}^t$ and $a_i \in \{0,1\}$, then we say that the $i$-th component of $\bar a$ is {\em defined}. 
\begin{itemize}
\item ${\sf Undef}(\bar u) := \neg \exists \bar v (\bar v \subset \bar u)$. That is, ${\sf Undef}$ defines the set that only consists of the tuple $\{\bot\}^{t}$ in which all components are undefined. 
\item ${\sf Single}(\bar u) := \forall \bar v (\bar v \subset \bar u \, \rightarrow \, {\sf Undef}(\bar v))$. 
That is, ${\sf Single}$ defines the set that consists precisely of those tuples in 
$\{0,1,\bot\}^{t}$ which have at most one component that is defined. 
%\item ${\sf Full}(\bar u) := \neg \exists \bar v (\bar u \subset \bar v)$. That is, ${\sf Full}$ defines the set of tuples in $\{0,1\}^t$; i.e, those tuples without undefined components. 
\item $(\bar u \sqcup \bar v = \bar z) := (\bar u \subseteq \bar z) \wedge (\bar v \subseteq \bar z) \wedge \neg \exists \bar w \big((\bar u \subseteq \bar z) \wedge (\bar v \subseteq \bar z) \wedge (\bar z \subset \bar w)\big)$. That is, $\bar z$, if it exists, is the {\em join} of $\bar u$ and $\bar v$. 
\item $(\bar u \sqcap \bar v = \bar z) := (\bar z \subseteq \bar u) \wedge (\bar z \subseteq \bar v) \wedge \neg \exists \bar w \big((\bar z \subseteq \bar u) \wedge (\bar z \subseteq \bar v) \wedge (\bar w \subset \bar z)\big)$. That is, $\bar z$ is the {\em meet} of $\bar u$ and $\bar v$ (which always exists). 
\item ${\sf Comp}(\bar u,\bar v) := \exists \bar w \exists z ({\sf Undef}(\bar z) \, \wedge \, \bar u \sqcup \bar v = \bar z \, \wedge \, \bar u \sqcap \bar v = \bar w)$.   
That is, ${\sf Comp}$ defines the pairs $(\bar a,\bar b)$ 
of tuples in $\{0,1,\bot\}^t \times \{0,1,\bot\}^t$ such that no component that is defined in $\bar a$ is also defined in $\bar b$, and viceversa. In fact, assume 
for the sake of contradiction that this is not the case. By symmetry, we only have to consider two cases.
\begin{itemize}
\item There is an $i \leq t$ with $a_i = 1$ and $b_i = 0$. Then the join of $\bar a$ and $\bar b$ does not exist. 
\item There is an $i \leq t$ with $a_i  = b_i = 1$. Then the $i$-th component of the meet of $\bar a$ and $\bar b$ is 1, and hence $\bar a \sqcap \bar b = \{\bot\}^t$. 
\end{itemize} 
\item ${\sf MaxComp}(\bar u,\bar v) := {\sf Comp}(\bar u,\bar v) \, \wedge \, \neg \exists \bar w \big((\bar v \subseteq \bar w) \wedge {\sf Comp}(\bar u,\bar w)\big)$.    
That is, ${\sf MaxComp}$ defines the pairs $(\bar a,\bar b)$ such that the components that are defined in $\bar a$ are precisely the ones that are undefined in $\bar b$, and viceversa.  
%Notice, by definition, that if $(\bar a,\bar b)$ belongs to the interpretation of ${\sf MaxComp}$ then $\bar a \sqcup \bar b$ exists 
%and belongs to the interpretation of ${\sf Full}$. 
\item ${\sf Rel}(\bar u,\bar v) := \neg \exists \bar w \big((\bar w \subseteq \bar v)  \, \wedge \, {\sf Single}(\bar w) \, \wedge\, {\sf Comp}(\bar u,\bar w)\big)$. 
That is, ${\sf Rel}$ defines the pairs $(\bar a,\bar b)$ 
of tuples in $\{0,1,\bot\}^t \times \{0,1,\bot\}^t$ such that every component that is defined in $\bar b$ is also defined in $\bar a$.
\item ${\sf MaxRel}(\bar u,\bar v) := {\sf Rel}(\bar u,\bar v) \, \wedge \, \neg \exists \bar w \big((\bar v \subset \bar w) \wedge {\sf Rel}(\bar u,\bar w)\big)$.    
That is, ${\sf MaxRel}$ defines the pairs $(\bar a,\bar b)$ such that the components defined in $\bar a$ and in $\bar b$ are the same.  
Notice, by definition, that if $(\bar a,\bar b)$ belongs to the interpretation of ${\sf MaxComp}$ then $\bar a \sqcup \bar b$ exists 
and belongs to the interpretation of ${\sf Full}$. 
\end{itemize}

We now explain the reduction. 
Consider an instance of the problem {\sc Positive One-in-Three 3Sat}, which we know it is {\sc NP}-complete. 
Recall that such an instance consists of a propositional formula 
$\phi = C_1 \wedge \ldots \wedge C_m$ in 3CNF in which each clause $C_i$, for $i \leq m$, is a disjunction of exactly three propositional 
variables from a set $\{x_1,\dots,x_n\}$. We want to check if there 
is an assignment $\sigma : \{x_1,\dots,x_n\} \to \{0,1\}$ such that, for each clause $C_i$ with $i \leq m$, 
there is exactly one variable in $C_i$ that is assigned value 1 under $\sigma$.   
We assume, without loss of generality, that $m = 2^q$ for some integer $q > 0$.  

With each $V \subseteq \{x_1,\dots,x_n\}$, we associate a different tuple $\bar V \in \{\bot\}^q \times \{0,1\}^n$ defined as $(\bot,\ldots,\bot,\chi_V)$, where $\chi_V \in \{0,1\}^n$ is the 
tuple whose $i$-th component is a 1, if $x_i \in V$, and it is a 0 otherwise. 
Analogously, with each clause $C_j$, for $j \leq m$, we associate a different tuple $\bar C_j \in \{0,1\}^q \times \{\bot\}^n$ defined as $([j-1],\bot,\ldots,\bot)$, 
where $[j-1] \in \{0,1\}^q$ is the 
binary encoding of $j-1$. Furthermore, we write $(\bar C_j,\bar V)$ for the instance $([j-1],\chi_V) \in \{0,1\}^{q+n}$. Notice that 
$\bar C_j \sqcup \bar V = (\bar C_j,\bar V)$. 
%$(\bar x_i,\bar C_j)$ is the only tuple $\bar v \in \{0,1\}^{p+q}$ which satisfies $\bar x_i,\bar C_j \subseteq \bar v$.   

From our input instance we build a decision tree $\D_\phi$, of arity $(q+n)$, that accepts precisely the tuples $(\bar C_j,\bar V) \in \{0,1\}^{q+n}$ satisfying that 
$V$ contains exactly 
one propositional variable from $C_j$. 

\begin{claim}
The decision tree $\D_\phi$ can be constructed in polynomial time from our input instance.
\end{claim}

\begin{proof} 
We build a complete decision tree for the first $q$ variables, which is of size $O(m)$ and thus polynomial on the input.  
For each $j \leq m$, we extend the leaf representing $[j-1]$ with a decision tree of depth three which checks if $V$ contains exactly one of the propositional variables in 
$C_j$. This decision tree is defined over the propositional variables in $C_j$. 
As an example, if $C_j = x_1 \wedge x_3 \wedge x_7$, then the decision tree first tests for the value of $x_1$. If $x_1 = 1$, it checks that $x_3 = x_7 = 0$. 
If $x_1 = 0$, it checks if either $x_3 = 1$ or $x_7 = 1$.  
\end{proof}

We now define a \FO\ formula
%\begin{multline*}
$$
\phi(\bar u) \ := \ \exists \bar v \, \bigg( \, {\sf MaxRel}(\bar u,\bar v) \, \wedge \, \forall \bar w \forall \bar z \big({\sf MaxComp}(\bar u,\bar w) \wedge (\bar v \sqcup \bar w = \bar z) \, \rightarrow \, \pos(\bar z) \big) \, \bigg).  
$$
%
%\forall \bar v \bigg( \, {\sf MaxComp}(\bar u,\bar v) \, \rightarrow \, \\ \exists! \bar w 
%\big(\, {\sf MaxRel}(\bar u,\bar w) \wedge \forall \bar z (\bar w \cap \bar u' = \bar z \rightarrow \pos(\bar z)) \, \big) \, \bigg). 
%\end{multline*}

Finally, we prove that our original instance $C_1 \wedge \ldots \wedge C_m$ of {\sc Positive One-in-Three 3Sat} has a solution if, and only if, 
$\astruct_{\D_\phi} \models \phi(\bar X)$, for $X = \{x_1,\dots,x_n\}$. (Recall that $\bar X \in \{\bot\}^q \times \{0,1\}^n$ is the tuple $(\bot,\ldots,\bot,\chi_X)$). 

Assume first that $C_1 \wedge \ldots \wedge C_m$ has a solution. This is an assignment $\sigma : \{x_1,\dots,x_n\} \to \{0,1\}$ that satisfies exactly one variable per clause. 
Let $V$ be the set of all variables in $\{x_1,\dots,x_n\}$ that are assigned value 1 under $\sigma$. 
We show that, in order to satisfy $\phi(\bar X)$ in $\astruct_{\D_\phi}$, 
the existentially quantified variable $\bar v$ can be witnessed by the tuple $\bar V \in \{\bot\}^q \times \{0,1\}^n$. 
In fact, the components which are defined in $\bar V$ and in $\bar X$ are the same, and hence 
$(\bar X,\bar V)$ belongs to the interpretation of ${\sf MaxRel}$. 
%Moreover, the set defined by the formula $\bar a  \subseteq \bar u' \wedge {\sf MaxRel}(\bar x_1,\bar u')$ over $\astruct_{\D_\phi}$ is precisely $\{\bar x_i \mid x_i \in X\}$. 
Now, take an arbitrary tuple $\bar a \in \{0,1,\bot\}^{q+n}$ 
satisfying $\astruct_{\D_\phi} \models {\sf MaxComp}(\bar X,\bar a)$. 
By definition, then, $\bar a \in \{0,1\}^q \times \{\bot\}^n$, and hence $\bar a = \bar C_j$ for some $j \leq m$. 
By hypothesis, 
there exists exactly one propositional variable in $C_j$ receiving value $1$ under $\sigma$. 
Hence, there exists exactly one propositional variable in $C_j$ that belongs to $V$. We conclude that $(\bar C_j \cup \bar V) = (\bar C_j,\bar V)$ belongs to the interpretation of predicate 
$\pos$ in $\astruct_{\D_\phi}$, which implies that $\astruct_{\D_\phi} \models \phi(\bar X)$. 
%
%there is exactly one tuple $\bar x$ in the interpretation of  
%%$\bar a  \subseteq \bar u' \wedge {\sf MaxRel}(\bar x_1,\bar u')$ over $\astruct_{\D_\phi}$ for which it holds that the meet of $\bar x$ and $\bar C_j$ is a positive instance of $\D_\phi$. This tuple $\bar x$ is 
%%precisely $\bar x_i$.

Assume now that $\astruct_{\D_\phi} \models \phi(\bar X)$. Let $\bar a \in \{0,1,\bot\}^{q+n}$ be a tuple for which 
$$\astruct_{\D_\phi} \, \models \, {\sf MaxRel}(\bar X,\bar a) \, \wedge \, \forall \bar w \forall \bar z\big({\sf MaxComp}(\bar X,\bar w) \wedge (\bar a \sqcup \bar w = \bar z) \, \rightarrow \, \pos(\bar z) \big).$$  Since ${\sf MaxRel}(\bar X,\bar a)$ holds in $\astruct_{\D_\phi}$, it must be the case that $\bar a \in \{\bot\}^q \times \{0,1\}^n$, and hence $\bar a = \bar V$ for some 
$V \subseteq \{x_1,\dots,x_n\}$. We define assignment $\sigma :  \{x_1,\dots,x_n\} \to \{0,1\}$ such that $\sigma(x_i) = 1$ if, and only if, $x_i \in V$. 
Take an arbitrary clause $C_j$, for $j \leq m$. Hence, $\astruct_{\D_\phi} \models \forall \bar z\big({\sf MaxComp}(\bar X,\bar C_j) \wedge (\bar V \sqcup \bar C_j = \bar z) \, \rightarrow \, \pos(\bar z) \big)$. Since $(\bar X,\bar C_j)$ satisfies ${\sf MaxComp}$, 
we obtain that$(\bar C_j,\bar V)$ belongs to the interpretation of $\pos$ in $\astruct_{\D_\phi}$. Hence by definition, there is exactly one variable from $C_j$ in $V$. We conclude that there exists exactly one variable from $C_j$ that is assigned value 1 under $\sigma$. 
